# Supplementary material for: `Interaction annealing' to determine effective quantized valence and orbital structure: an illustration with ferro-orbital order in WTe$_2$
Source: arXiv:2407.03319 source file (2025-12-17)
Supplement: Supplementary file 1 [file Supp_Interaction_annealing_strategy.pdf]

# Supplemental materials

Ruoshi Jiang, Fangyuan Gu, and Wei Ku

## 1. Obtaining low-energy effective Hamiltonian via numerical canonical transformation

Low-energy effective theory is one of the most effective means to capture and understand the key physics of a quantum system within a well-defined energy scale. Conceptually, it can be rigorously constructed by integrating out the high-energy states in the path integral formulation. Equivalently, it can also be derived by decoupling the remaining low-energy states from the high ones. Specifically, one finds a unitary transformation[S1, S2],  $\mathcal{U}[\{c_i, c_i^\dagger\}]$ , of the second quantized basis,  $c_i$ , spanning the one-body space indexed by  $i$ ,

$$\tilde{c}_i = \mathcal{U}^\dagger c_i \mathcal{U}, \quad (\text{S1})$$

such that the Hamiltonian has a ‘block diagonal’ form,  $\tilde{H}$ , in the new ‘many-body dressed’ representation,  $\tilde{c}_i$  (freeing the low-energy subspace from the influence of the high-energy subspace),

$$H[\{c_i, c_i^\dagger\}] = \tilde{H}[\{\tilde{c}_i, \tilde{c}_i^\dagger\}]. \quad (\text{S2})$$

Given

$$\begin{aligned} \tilde{H}[\{\tilde{c}_i, \tilde{c}_i^\dagger\}] &= \tilde{H}[\{\mathcal{U}^\dagger c_i \mathcal{U}, \mathcal{U}^\dagger c_i^\dagger \mathcal{U}\}] \\ &= \mathcal{U}^\dagger \tilde{H}[\{c_i, c_i^\dagger\}] \mathcal{U}, \end{aligned} \quad (\text{S3})$$

the unitary transformation  $\mathcal{U}$  can thus be found by demanding

$$\tilde{H}[\{c_i, c_i^\dagger\}] = \mathcal{U} H[\{c_i, c_i^\dagger\}] \mathcal{U}^\dagger, \quad (\text{S4})$$

to possess the desired block diagonal form.

As a simple illustration for such an emergent structure, consider a two-site Hubbard model,

$$H = -t \sum_{\mu} (c_{1\mu}^\dagger c_{2\mu} + c_{2\mu}^\dagger c_{1\mu}) + U (c_{1\uparrow}^\dagger c_{1\downarrow}^\dagger c_{1\downarrow} c_{1\uparrow} + c_{2\uparrow}^\dagger c_{2\downarrow}^\dagger c_{2\downarrow} c_{2\uparrow}),$$

containing two electrons, where  $t$  denotes the kinetic hopping between site 1 and 2,  $\mu$  the quantized spin index ( $\uparrow, \downarrow$ ), and  $U$  the charging energy when both electrons are located in the same site. Let’s examine the low-energy effective theories of this system in the two representative regimes of such a system with  $t \ll U$  and  $t \gg U$ .

In the regime of  $t \ll U$ , states with doubly occupied orbitals are the high-energy ones, as shown in the left panel of Fig S1(a). By defining the unitary transformation  $\mathcal{U} = \exp\left(\frac{\theta}{2} \sum_{\mu} \frac{1}{2} (c_{1\mu}^\dagger c_{2\mu} - c_{2\mu}^\dagger c_{1\mu}) (n_{2\bar{\mu}} - n_{1\bar{\mu}})\right)$ , and decoupling these states from the remaining low-energy sector (constrained by  $\tilde{c}_{1\uparrow}^\dagger \tilde{c}_{1\downarrow}^\dagger = \tilde{c}_{2\uparrow}^\dagger \tilde{c}_{2\downarrow}^\dagger = 0$ ), the resulting low-energy effective theory,

$$\tilde{H}^{(t \ll U)} = \tilde{J}_{12} (\tilde{\mathbf{S}}_1 \cdot \tilde{\mathbf{S}}_2 - \frac{1}{4}), \quad (\text{S5})$$

contains only singly occupied sites  $i = 1, 2$  with anti-ferromagnetic super-exchange  $\tilde{J}_{12} = \frac{U}{2} (\cos \theta - 1) + 2t \sin \theta = \frac{1}{2} (\sqrt{U^2 + (4t)^2} - U)$  between them, without charge degree of freedom, where  $\tilde{\mathbf{S}}_i = \sum_{\mu\nu} \tilde{c}_{i\mu}^\dagger \sigma_{\mu\nu} \tilde{c}_{i\nu}$  denotes the total spin via the standard Pauli matrices,  $\sigma_{\mu\nu}$ .

The dressed particles are  $\tilde{c}_{i\mu}^\dagger = \mathcal{U}^\dagger c_{i\mu}^\dagger \mathcal{U}$  at site  $i$ .

$$\tilde{c}_{i\mu}^\dagger = c_{i\mu}^\dagger + (\sin \frac{\theta}{2}) \frac{1}{2} [c_{i\mu}^\dagger (c_{i\bar{\mu}}^\dagger c_{i'\bar{\mu}} - c_{i'\bar{\mu}}^\dagger c_{i\bar{\mu}}) + c_{i'\bar{\mu}}^\dagger (n_{i'\bar{\mu}} - n_{i\bar{\mu}})] + (\cos \frac{\theta}{2} - 1) \frac{1}{2} [c_{i'\mu}^\dagger (c_{i\bar{\mu}}^\dagger c_{i'\bar{\mu}} + c_{i'\bar{\mu}}^\dagger c_{i\bar{\mu}}) + c_{i\bar{\mu}}^\dagger (n_{i\bar{\mu}} + n_{i'\bar{\mu}})], \quad (\text{S6})$$

where  $\tan \theta = \frac{4t}{U}$ .

On the other hand, in the  $t \gg U$  regime, naturally one should first account for the rapid dynamics of one-body kinetic processes between the two sites, by representing  $H$  using the bonding orbital,  $b_\mu^\dagger \equiv \frac{1}{\sqrt{2}} (c_{1\mu}^\dagger + c_{2\mu}^\dagger)$ , and the anti-bonding orbital,  $a_\mu^\dagger \equiv \frac{1}{\sqrt{2}} (c_{1\mu}^\dagger - c_{2\mu}^\dagger)$  that diagonalize the  $t$ -associated one-body part of  $H$ ,

$$H = t \sum_{\mu} (-b_\mu^\dagger b_\mu + a_\mu^\dagger a_\mu) + \frac{U}{2} \prod_{\mu} (b_\mu^\dagger b_\mu + a_\mu^\dagger a_\mu) + \frac{U}{2} \prod_{\mu} (a_\mu^\dagger b_\mu + b_\mu^\dagger a_\mu). \quad (\text{S7})$$

(a)  $t \ll U$

$$\begin{array}{l}
1\uparrow\uparrow2 \\
1\uparrow\downarrow2 \\
1\downarrow\uparrow2 \\
1\downarrow\downarrow2 \\
1\uparrow\uparrow2 \\
1\downarrow\downarrow2
\end{array}
\begin{array}{c}
\left( \begin{array}{cccc|cc}
0 & 0 & 0 & 0 & -t & -t \\
0 & 0 & 0 & 0 & t & t \\
0 & 0 & 0 & 0 & 0 & 0 \\
0 & 0 & 0 & 0 & 0 & 0 \\
-t & t & 0 & 0 & U & 0 \\
-t & t & 0 & 0 & 0 & U
\end{array} \right)
\end{array}
\longleftrightarrow
\begin{array}{c}
\left( \begin{array}{cccc|cc}
-\frac{\tilde{J}_{12}}{2} & \frac{\tilde{J}_{12}}{2} & 0 & 0 & 0 & 0 \\
\frac{\tilde{J}_{12}}{2} & -\frac{\tilde{J}_{12}}{2} & 0 & 0 & 0 & 0 \\
0 & 0 & 0 & 0 & 0 & 0 \\
0 & 0 & 0 & 0 & 0 & 0 \\
0 & 0 & 0 & 0 & \tilde{U} & \frac{\tilde{J}_{12}}{2} \\
0 & 0 & 0 & 0 & \frac{\tilde{J}_{12}}{2} & \tilde{U}
\end{array} \right)
\end{array}$$

(b)  $t \gg U$

$$\begin{array}{l}
\uparrow\uparrow b \\
\uparrow\downarrow b \\
\downarrow\uparrow b \\
\downarrow\downarrow b \\
\uparrow\uparrow b \\
\uparrow\downarrow b
\end{array}
\begin{array}{c}
\left( \begin{array}{cccc|c}
-2t + \frac{U}{2} & 0 & 0 & 0 & \frac{U}{2} \\
0 & \frac{U}{2} & -\frac{U}{2} & 0 & 0 \\
0 & -\frac{U}{2} & \frac{U}{2} & 0 & 0 \\
0 & 0 & 0 & 0 & 0 \\
0 & 0 & 0 & 0 & 0 \\
\frac{U}{2} & 0 & 0 & 0 & 2t + \frac{U}{2}
\end{array} \right)
\end{array}
\longleftrightarrow
\begin{array}{c}
\left( \begin{array}{cccc|c}
2\tilde{\epsilon}_b & 0 & 0 & 0 & 0 \\
0 & \frac{\tilde{J}_{ba}}{2} & -\frac{\tilde{J}_{ba}}{2} & 0 & 0 \\
0 & -\frac{\tilde{J}_{ba}}{2} & \frac{\tilde{J}_{ba}}{2} & 0 & 0 \\
0 & 0 & 0 & 0 & 0 \\
0 & 0 & 0 & 0 & 0 \\
0 & 0 & 0 & 0 & \tilde{E}_a
\end{array} \right)
\end{array}$$

FIG. S1. Illustration of the emergent effective description with quantized valence, orbital, and spin structures, using the first-quantized representation of the two-site Hubbard model in its two regimes. (a) interaction dominant regime  $t \ll U$ : In this case, the emerged lower energy effective Hamiltonian is  $H^{(t \ll U)} = \tilde{J}_{12}(\tilde{\mathbf{S}}_1 \cdot \tilde{\mathbf{S}}_2 - \frac{1}{4})$  with anti-ferromagnetic coupling  $\tilde{J}_{12} = \frac{1}{2}(\sqrt{U^2 + (4t)^2} - U)$ , featuring a singlet ground state. (b) kinetic dominant regime  $t \gg U$ : The emerged lower energy effective Hamiltonian (right matrix) is  $\tilde{H}^{(t \gg U)} = \sum_{\mu} (\tilde{\epsilon}_b \tilde{b}_{\mu}^{\dagger} \tilde{b}_{\mu} + \tilde{\epsilon}_a \tilde{a}_{\mu}^{\dagger} \tilde{a}_{\mu}) - \tilde{J}_{ba} \tilde{\mathbf{S}}_b \cdot \tilde{\mathbf{S}}_a$ , with the ferromagnetic coupling  $\tilde{J}_{ba} = U$  and the emergent onsite energy  $\tilde{\epsilon}_b = -\frac{1}{4}(\sqrt{(4t)^2 + U^2} - U)$ ,  $\tilde{\epsilon}_a = -\tilde{\epsilon}_b + \frac{\tilde{J}_{ba}}{4}$ ,  $\tilde{E}_a = \frac{1}{2}(\sqrt{(4t)^2 + U^2} + U)$ , featuring the ground state with double occupancy in the bonding orbital.

For easier visualization, the left panel of Fig. S1(b) represents  $H$  in the corresponding many-body basis. Intuitively, the state with both electrons occupying the anti-bonding orbital has a very high energy. One can thus treat it as the high-energy state and decouple it from the more relevant low-energy subspace, via a unitary transformation  $\mathcal{U} = \exp\left(\frac{\phi}{2}(a_{\uparrow}^{\dagger} a_{\downarrow}^{\dagger} b_{\downarrow} b_{\uparrow} - b_{\uparrow}^{\dagger} b_{\downarrow}^{\dagger} a_{\downarrow} a_{\uparrow})\right)$  of the second quantized basis

$$\begin{aligned}
\tilde{b}_{\mu}^{\dagger} &= b_{\mu}^{\dagger} - (\sin \frac{\phi}{2}) a_{\mu}^{\dagger} a_{\bar{\mu}}^{\dagger} b_{\bar{\mu}} + (\cos \frac{\phi}{2} - 1) b_{\mu}^{\dagger} b_{\bar{\mu}}^{\dagger} b_{\bar{\mu}}, \\
\tilde{a}_{\mu}^{\dagger} &= a_{\mu}^{\dagger} + (\sin \frac{\phi}{2}) b_{\mu}^{\dagger} b_{\bar{\mu}}^{\dagger} a_{\bar{\mu}} + (\cos \frac{\phi}{2} - 1) a_{\mu}^{\dagger} a_{\bar{\mu}}^{\dagger} a_{\bar{\mu}},
\end{aligned} \tag{S8}$$

where  $\tan \phi = \frac{U}{4t}$ .

As represented in the many-body basis of the dressed particles shown in the right panel of Fig. S1(b), the resulting low-energy effective Hamiltonian (constrained by  $\tilde{a}_{\uparrow}^{\dagger} \tilde{a}_{\downarrow}^{\dagger} = 0$ ),

$$\tilde{H}^{(t \gg U)} = \sum_{\mu} (\tilde{\epsilon}_b \tilde{b}_{\mu}^{\dagger} \tilde{b}_{\mu} + \tilde{\epsilon}_a \tilde{a}_{\mu}^{\dagger} \tilde{a}_{\mu}) - \tilde{J}_{ba} \tilde{\mathbf{S}}_b \cdot \tilde{\mathbf{S}}_a, \tag{S9}$$

has instead an emergent ferromagnetic inter-orbital Hund's coupling of strength  $\tilde{J}_{ba} = U$  and the emergent onsite energy  $\tilde{\epsilon}_b = -t \cos \phi + \frac{U}{4}(1 - \sin \phi) = -\frac{1}{4}(\sqrt{(4t)^2 + U^2} - U)$  and  $\tilde{\epsilon}_a = -\tilde{\epsilon}_b + \frac{\tilde{J}_{ba}}{4}$ . Here,  $\tilde{\mathbf{S}}_b = \sum_{\mu\nu} \tilde{b}_{\mu}^{\dagger} \sigma_{\mu\nu} \tilde{b}_{\nu}$  and  $\tilde{\mathbf{S}}_a$  denotes the spin in the effective bonding and anti-bonding orbitals.

One sees that in either case above, the low-energy dynamics can be *exactly* described by an effective theory containing only *quantized* charge, orbital, and spin degrees of freedom. In essence, it is the bifurcating choice of such low-energy effective description that produces the rich complex behaviors of correlated materials [S3, S4].

## 2. Computational details of density functional calculation

Our first-principles calculations were performed using density functional theory (DFT)-based [S5, S6] WIEN2k package with the spin-polarized LDA+ $U$  [S7, S8] and the linearized augmented plane wave (LAPW) [S9] implementation [S10]. Monkhorst-Pack  $k$ -point grids for Brillouin zone sampling are set to  $9 \times 16 \times 4$  and  $9 \times 17 \times 4$  for bulk WTe<sub>2</sub> with  $1T$  and  $T_d$  structures, respectively. WTe<sub>2</sub> crystallizes in an orthorhombic Bravais lattice, with a  $T_d$  structure and space group  $Pmn21$  (No. 31). We used the experimental lattice constants reported by Brown *et al.* [S11],  $a = 6.28\text{\AA}$ ,  $b = 3.50\text{\AA}$ ,  $c = 14.07\text{\AA}$ , which were also confirmed by other experiments [S12]. As the higher-symmetry  $1T$  structure has not been observed in experiments, we built the structure with the same interlayer thickness as the experimental  $T_d$  structure and optimized the intralayer lattice parameters through atomic relaxation. The lattice constants used for calculations in this work are  $a = 6.06\text{\AA}$ ,  $b = 3.50\text{\AA}$ ,  $c = 14.07\text{\AA}$ .

In the interaction annealing process, we set the effective  $U$  on W  $d$ -orbitals within the range of 3 – 20 eV. The ‘heat up’ and ‘cool down’ processes correspond to smoothly increasing and decreasing the interaction strength  $U$  in 0.2 eV steps with a mix factor of 0.05.

## 3. One-body density matrix $\rho_{nn'}$ among the local W $t_{2g}$ orbitals

At the high- $U$  ( $\sim 20\text{eV}$ ) regime, one finds many stable structures in the LDA+ $U$  calculations, all with distinct well-defined ionic valence, orbital, and spin structures. In order to reveal the potential spontaneous symmetry breaking of the system, the idealized  $1T$  structure of higher symmetry with doubled W in one unit cell is thus built. Table S1 lists the one-body density matrix  $\rho_{nn'}$  among the local  $t_{2g}$  orbitals of two W atoms with index  $n$  for different  $U \sim 20\text{eV}$  configurations in  $1T$  structure.

## 4. Stable electronic state via electron-lattice coupling in $T_d$ structure

With the help of lattice distortion towards lower symmetry, which is consistent with the symmetry-broken electronic state, this electronic state would be further stabilized. Fig. S2 shows the stable configuration of WTe<sub>2</sub> and its adiabatic connection upon ‘heating up’ the interaction strength  $U$ . As  $U$  slowly increases from the realistic value  $\sim 3\text{eV}$  to large limit  $\sim 20\text{eV}$ , the configuration is OP2 with FO2 order, corresponding to the two electrons both occupying one of the two degenerate orbitals  $eg_2''$  with long-range ferro-orbital order. Table S2 lists the one-body density matrix  $\rho_{nn'}$  among the local W  $t_{2g}$  orbitals with index  $n$  in  $T_d$  lattice structure. For a realistic strength of intra-atomic interaction  $U \sim 3\text{eV}$ , the upper part of the table shows fractional occupation in all three orbitals (c.f. the diagonal elements) due to strong quantum charge fluctuation. The lower part gives the  $\rho_{nn'}$  for OP2(FO2) at high- $U$ , one of the three surviving OP2 configurations upon interaction annealing of the  $1T$  structure. Upon diagonalizing  $\rho_{nn'}$ , this configuration contains only one occupied orbital  $e_{g2}''$ . Both cases shown here have identical  $\rho_{nn'}$  for the up- and down-spin channels.

TABLE S1. One-body density matrix  $\rho_{nn'}$  among the local W  $t_{2g}$  orbitals with index  $n$  for different  $U \sim 20\text{eV}$  configurations in  $1T$  structure.

| $\rho_{nn'}$ | W(1)- $\uparrow$ |           |           | W(1)- $\downarrow$ |           |           | W(2)- $\uparrow$ |           |           | W(2)- $\downarrow$ |           |           |
|--------------|------------------|-----------|-----------|--------------------|-----------|-----------|------------------|-----------|-----------|--------------------|-----------|-----------|
|              | $a_g$            | $e'_{g1}$ | $e'_{g2}$ | $a_g$              | $e'_{g1}$ | $e'_{g2}$ | $a_g$            | $e'_{g1}$ | $e'_{g2}$ | $a_g$              | $e'_{g1}$ | $e'_{g2}$ |
| LS2          | 0.81             | 0.00      | 0.00      | 0.81               | 0.00      | 0.00      | 0.81             | 0.00      | 0.00      | 0.81               | 0.00      | 0.00      |
|              | 0.00             | 0.06      | 0.00      | 0.00               | 0.06      | 0.00      | 0.00             | 0.06      | 0.00      | 0.00               | 0.06      | 0.00      |
|              | 0.00             | 0.00      | 0.06      | 0.00               | 0.00      | 0.06      | 0.00             | 0.00      | 0.06      | 0.00               | 0.00      | 0.06      |
| HS3(FM)      | 0.83             | 0.00      | 0.00      | 0.03               | 0.00      | 0.00      | 0.83             | 0.00      | 0.00      | 0.03               | 0.00      | 0.00      |
|              | 0.00             | 0.81      | 0.00      | 0.00               | 0.02      | 0.00      | 0.00             | 0.81      | 0.00      | 0.00               | 0.02      | 0.00      |
|              | 0.00             | 0.00      | 0.81      | 0.00               | 0.00      | 0.02      | 0.00             | 0.00      | 0.81      | 0.00               | 0.00      | 0.02      |
| HS3(AFM)     | 0.82             | 0.00      | 0.00      | 0.03               | 0.00      | 0.00      | 0.03             | 0.00      | 0.00      | 0.82               | 0.00      | 0.00      |
|              | 0.00             | 0.81      | 0.00      | 0.00               | 0.02      | 0.00      | 0.00             | 0.02      | 0.00      | 0.00               | 0.81      | 0.00      |
|              | 0.00             | 0.00      | 0.81      | 0.00               | 0.00      | 0.02      | 0.00             | 0.00      | 0.02      | 0.00               | 0.00      | 0.81      |
| OP2(FO1)     | 0.06             | -0.06     | -0.06     | 0.06               | -0.07     | -0.07     | 0.06             | -0.05     | -0.05     | 0.06               | -0.07     | -0.07     |
|              | -0.06            | 0.44      | 0.36      | -0.07              | 0.43      | 0.37      | -0.05            | 0.44      | 0.37      | -0.07              | 0.43      | 0.37      |
|              | -0.06            | 0.36      | 0.44      | -0.07              | 0.37      | 0.43      | -0.05            | 0.37      | 0.44      | -0.07              | 0.37      | 0.43      |
| OP2(FO2)     | 0.06             | 0.02      | 0.02      | 0.06               | 0.01      | 0.01      | 0.06             | 0.02      | 0.02      | 0.06               | 0.01      | 0.01      |
|              | 0.02             | 0.45      | -0.36     | 0.01               | 0.44      | -0.37     | 0.02             | 0.45      | -0.36     | 0.01               | 0.44      | -0.36     |
|              | 0.02             | -0.36     | 0.45      | 0.01               | -0.37     | 0.44      | 0.02             | -0.36     | 0.45      | 0.01               | -0.36     | 0.44      |
| OP2(AFO)     | 0.06             | 0.06      | 0.06      | 0.06               | 0.06      | 0.06      | 0.07             | 0.01      | 0.01      | 0.06               | 0.01      | 0.01      |
|              | 0.06             | 0.43      | 0.36      | 0.06               | 0.43      | 0.36      | 0.01             | 0.45      | -0.36     | 0.01               | 0.45      | -0.36     |
|              | 0.06             | 0.36      | 0.43      | 0.06               | 0.36      | 0.43      | 0.01             | -0.36     | 0.45      | 0.01               | -0.36     | 0.45      |
| OP3(FO1)     | 0.80             | -0.02     | -0.02     | 0.03               | -0.03     | -0.03     | 0.80             | -0.01     | -0.01     | 0.03               | -0.03     | -0.03     |
|              | -0.02            | 0.40      | 0.36      | -0.03              | 0.38      | 0.35      | -0.01            | 0.40      | 0.36      | -0.03              | 0.38      | 0.34      |
|              | -0.02            | 0.36      | 0.40      | -0.03              | 0.35      | 0.38      | -0.01            | 0.36      | 0.40      | -0.03              | 0.34      | 0.38      |
| OP3(FO2)     | 0.77             | 0.11      | 0.11      | 0.03               | 0.00      | 0.00      | 0.77             | 0.11      | 0.11      | 0.03               | 0.00      | 0.00      |
|              | 0.11             | 0.42      | -0.35     | 0.00               | 0.37      | -0.34     | 0.11             | 0.42      | -0.35     | 0.00               | 0.37      | -0.34     |
|              | 0.11             | -0.35     | 0.42      | 0.00               | -0.34     | 0.37      | 0.11             | -0.35     | 0.42      | 0.00               | -0.34     | 0.37      |
| OP3(AFO)     | 0.81             | -0.01     | -0.01     | 0.03               | 0.01      | 0.01      | 0.79             | -0.08     | -0.08     | 0.03               | 0.00      | 0.00      |
|              | -0.01            | 0.41      | 0.37      | 0.01               | 0.38      | 0.35      | -0.08            | 0.42      | -0.36     | 0.00               | 0.38      | -0.35     |
|              | -0.01            | 0.37      | 0.41      | 0.01               | 0.35      | 0.38      | -0.08            | -0.36     | 0.42      | 0.00               | -0.35     | 0.38      |
| OP3(FO1+AFM) | 0.80             | -0.01     | -0.01     | 0.03               | -0.02     | -0.02     | 0.03             | -0.02     | -0.02     | 0.80               | -0.02     | -0.02     |
|              | -0.01            | 0.40      | 0.36      | -0.02              | 0.37      | 0.34      | -0.02            | 0.38      | 0.34      | -0.02              | 0.39      | 0.36      |
|              | -0.01            | 0.36      | 0.40      | -0.02              | 0.34      | 0.37      | -0.02            | 0.34      | 0.38      | -0.02              | 0.36      | 0.39      |
| OP3(FO2+AFM) | 0.77             | 0.11      | 0.11      | 0.03               | 0.00      | 0.00      | 0.03             | 0.00      | 0.00      | 0.77               | 0.11      | 0.11      |
|              | 0.11             | 0.41      | -0.35     | 0.00               | 0.38      | -0.35     | 0.00             | 0.39      | -0.35     | 0.11               | 0.41      | -0.34     |
|              | 0.11             | -0.35     | 0.41      | 0.00               | -0.35     | 0.38      | 0.00             | -0.35     | 0.39      | 0.11               | -0.34     | 0.41      |
| OP3(AFO+AFM) | 0.81             | -0.02     | -0.02     | 0.03               | 0.01      | 0.01      | 0.03             | 0.00      | 0.00      | 0.80               | -0.04     | -0.04     |
|              | -0.02            | 0.40      | 0.36      | 0.01               | 0.38      | 0.35      | 0.00             | 0.39      | -0.36     | -0.04              | 0.40      | -0.35     |
|              | -0.02            | 0.36      | 0.40      | 0.01               | 0.35      | 0.38      | 0.00             | -0.36     | 0.39      | -0.04              | -0.35     | 0.40      |

TABLE S2. One-body density matrix  $\rho_{nn'}$  among the local W  $t_{2g}$  orbitals with index  $n$  in  $T_d$  structure. For a realistic strength of intra-atomic interaction  $U \sim 3\text{eV}$ , the upper part of the table shows fractional occupation in all three orbitals (c.f. the diagonal elements) due to strong quantum charge fluctuation. The lower part gives the  $\rho_{nn'}$  for OP2(FO2) at high- $U$ , one of the three OP2 configurations. Upon diagonalizing  $\rho_{nn'}$ , this configuration contains only one occupied orbital  $e''_{g2}$ . Both cases shown here have identical  $\rho_{nn'}$  for the up- and down-spin channels.

| $\rho_{nn'}$           | $a_g$ | $e'_{g1}$ | $e'_{g2}$ |
|------------------------|-------|-----------|-----------|
| $U \sim 3 \text{ eV}$  | 0.37  | -0.02     | -0.02     |
|                        | -0.02 | 0.32      | -0.09     |
|                        | -0.02 | -0.09     | 0.32      |
| $U \sim 20 \text{ eV}$ | 0.11  | 0.01      | 0.01      |
|                        | 0.01  | 0.44      | -0.35     |
|                        | 0.01  | -0.35     | 0.44      |

  

| $\rho_{nn'}$           | $a_g$ | $e''_{g1}$ | $e''_{g2}$ |
|------------------------|-------|------------|------------|
| $U \sim 20 \text{ eV}$ | 0.11  | 0.01       | 0.01       |
|                        | 0.01  | 0.09       | 0          |
|                        | 0.01  | 0          | 0.79       |

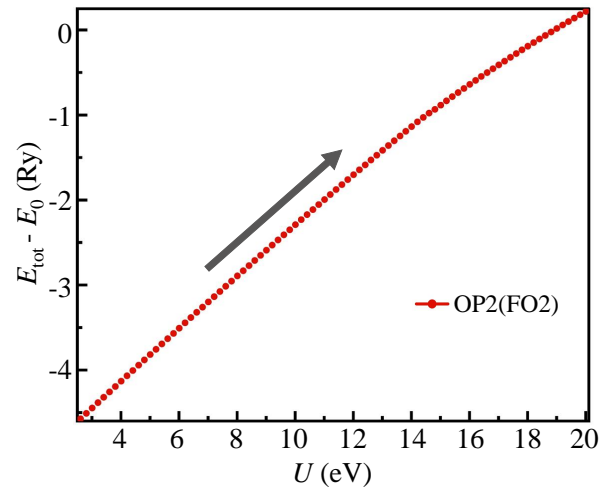

FIG. S2. (color online) Stable configuration of  $\text{WTe}_2$  and its adiabatic connection upon ‘heating up’ the interaction strength  $U$  in  $T_d$  structure. As  $U$  slowly increases from the realistic value  $\sim 3\text{eV}$  to large limit  $\sim 20\text{eV}$ , the configuration is clearly the OP2 with FO2 ordering, corresponding to two electrons both occupying one of the two degenerate orbitals  $eg'_2$  with long-range ferro-orbital order.

- 
- [S1] K. Chao, J. Spalek, and A. Oles, Kinetic exchange interaction in a narrow s-band, *Journal of Physics C: Solid State Physics* **10**, L271 (1977).
  - [S2] S. White, Numerical canonical transformation approach to quantum many-body problems, *The Journal of Chemical Physics* **117** (2002).
  - [S3] E. Dagotto, Complexity in strongly correlated electronic systems, *Science* **309**, 257 (2005).
  - [S4] P. W. Anderson, More is different, *Science* **177**, 393 (1972).
  - [S5] P. Hohenberg and W. Kohn, Inhomogeneous electron gas, *Phys. Rev.* **136**, B864 (1964).
  - [S6] W. Kohn and L. J. Sham, Self-consistent equations including exchange and correlation effects, *Phys. Rev.* **140**, A1133 (1965).
  - [S7] V. I. Anisimov, I. V. Solovyev, M. A. Korotin, M. T. Czyżyk, and G. A. Sawatzky, Density-functional theory and nio photoemission spectra, *Phys. Rev. B* **48**, 16929 (1993).
  - [S8] A. I. Liechtenstein, V. I. Anisimov, and J. Zaanen, Density-functional theory and strong interactions: Orbital ordering in mott-hubbard insulators, *Phys. Rev. B* **52**, R5467 (1995).
  - [S9] D. J. Singh, *Planewaves, Pseudopotentials and the LAPW Method* (Springer New York, NY, New York, 2006).
  - [S10] P. Blaha, K. Schwarz, P. Sorantin, and S. Trickey, Full-potential, linearized augmented plane wave programs for crystalline systems, *Computer Physics Communications* **59**, 399 (1990).
  - [S11] B. E. Brown, The crystal structures of wte2 and high-temperature mote2, *Acta Crystallographica* **20**, 268 (1966).
  - [S12] C. Lee, E. Silva, L. Calderin, M. Nguyen, M. Hollander, B. Bersch, T. Mallouk, and J. Robinson, English (US) Tungsten ditelluride: A layered semimetal, *Scientific reports* **5**, 10.1038/srep10013 (2015).
